# Supplementary material for: A Feedback Capacity-Achieving Coding Scheme for the $(d,\infty)$-RLL Input-Constrained Binary Erasure Channel
Source: arXiv:2204.06780 source file (2022-04-14)
Supplement: Supplementary file 3 [file appendixc.tex]

In this section, we shall prove Proposition \ref{prop:lp} by showing that the maximization problem, therein, can be cast as an LP, and obtain an upper bound by considering the corresponding Lagrange dual.

\begin{proof}
First, we shall set up the LP. Similar to the approach in \cite{0k}, we choose the optimization variables to be $\mathbf{d}:= \left(P_{S,Q,X,Y}(s,v,x,y): (s,v,x,y)\in \mathscr{S}\times \mathscr{V}^{(d)}\times \mathscr{X}\times \mathscr{Y} \right)$, i.e., the probabilities of the edges of the $(S,Q)$-graph, $\mathscr{G}_{SQ}^{(d)}$. Note that for a given edge, $(s,v,x,y)$, the joint distribution can be written as $P(s,v,x,y) = P(s,v)P(x|s,v)P(y|x)$. 

We now put down three constraints that the optimization variables must satisfy:

\begin{enumerate}
	\item \emph{PMF}: The variables must form a valid pmf, and must hence sum to one. The corresponding constraint function is given by:
	\begin{equation}\label{eq:const1}
	h_1(\mathbf{d}):=\sum_{s,v,x,y} P(s,v,x,y).
	\end{equation}
	\item \emph{Stationarity}: We require that the marginal distribution, $P_{S,Q}(s,v) = \pi(s,v)$, for all $(s,v)\in \mathscr{S}\times \mathscr{V}^{(d)}$, where $\pi(\cdot)$ is the unique stationary distribution on the nodes of $\mathscr{G}_{SQ}^{(d)}$. Formally, the constraint function for each $(s,v)$ is given by:
	\begin{align}\label{eq:const2}
	h_i(\mathbf{d}):=\sum\limits_{(s^\prime,v^\prime,x^\prime,y^\prime)\in N^{-}(s,v)}&P(s^\prime,v^\prime,x^\prime,y^\prime)\\
	&\ -\sum\limits_{(s,v,x,y)\in N^{+}(s,v)}P(s,v,x,y),
	\end{align}
	where $i=2,\ldots,|\mathscr{S}\times \mathscr{V}^{(d)}|+1$ are indices corresponding to the nodes of $\mathscr{G}_{SQ}^{(d)}$. We use the notation $N^-(s,v)$ to denote the set of incoming edges into the node $(s,v)$, and $N^+(s,v)$ to denote the set of outgoing edges from $(s,v)$.  
	\item \emph{Erasure}: For the memoryless BEC, it holds that $P(Y=?|x) = P(Y=?|s,v,x) = \epsilon$, for all $(s,v,x)\in \mathscr{S}\times \mathscr{V}^{(d)}\times \mathscr{X}$. Hence, the corresponding constraint function is written as:
	\begin{equation}\label{eq:const3}
	h_i(\mathbf{d}):= \sum\limits_x P(s,v,x,?) - \epsilon \cdot \sum\limits_{(s,v,x,y)\in N^+(s,v)}P(s,v,x,y),
	\end{equation}
	where $i=|\mathscr{S}\times \mathscr{V}^{(d)}|+2,\ldots,2.|\mathscr{S}\times \mathscr{V}^{(d)}|+1$ are indices that correspond to the nodes of $\mathscr{G}_{SQ}^{(d)}$.
\end{enumerate}

Our optimization problem can then be written as:

\begin{align}\label{LP}
&\text{maximize}_\mathbf{d}\ f_0(\mathbf{d}):= \sum_{\mathbf{q}\in \mathscr{V}_{\text{DB}}^{(d)}} P(d,\mathbf{q},1,y)\\
&\text{subject to}\ f_1(\mathbf{d})=1,\\
&\quad \quad \quad \quad \  f_i(\mathbf{d})=0, \ i=1,\ldots, 2.|\mathscr{S}\times \mathscr{V}^{(d)}|+1, \notag\\
&\quad \quad \quad \quad \quad  \mathbf{d} \succcurlyeq 0, \notag
\end{align}

where the notation $\mathbf{a} \succcurlyeq \mathbf{b}$, for $\mathbf{a}, \mathbf{b} \in \mathbb{R}^n$, means that $a_i \geq b_i$, for all $i\in [n]$. Since the objective function, $f_0(\mathbf{d})$, and the constraint functions are all linear in the optimization variables, it is immediate that the optimization problem \eqref{LP} is a linear program.

For ease of notation, we shall represent our \emph{primal} LP \eqref{LP} in the standard form as:
\begin{align}\label{LP:std}
&\text{maximize}\ \mathbf{c}^T\mathbf{d}\\
&\text{subject to}\ A\mathbf{d} = \mathbf{b}, \notag\\
&\quad \quad \quad \quad \quad  \mathbf{d}\succcurlyeq 0, \notag
\end{align}
where $\mathbf{c}$ is a column vector of length $|\mathbf{d}|:=|\mathscr{S}\times \mathscr{V}^{(d)}\times \mathscr{X}\times \mathscr{Y}|$, whose co-ordinates are indexed by the edges, $(s,v,x,y)$, such that $c(d,\mathbf{q},1,y) = 1$, for $y\in \mathscr{Y}$, and $\mathbf{q}\in \mathscr{V}_{\text{DB}}^{(d)}$, and has $0$s at all other co-ordinates. The matrix $A$ has $r:= 2.|\mathscr{S}\times \mathscr{V}^{(d)}|+1$ rows, each corresponding to a constraint, and $|\mathbf{d}|$ columns, corresponding to the variables. Further, $\mathbf{b}$ is taken to be equal to $\mathbf{e}_1^{r}$.

The Lagrange dual of the standard form LP in \eqref{LP:std} is given by:
\begin{align}\label{LP:dual}
&\text{mimimize}\ \mathbf{b}^T\mathbf{u}\\
&\text{subject to}\ A^T\mathbf{u} \succcurlyeq \mathbf{c}, \notag
\end{align}
where $\mathbf{u}$ is a column vector of length $r$. Let us denote the maximum value of the primal LP, in \eqref{LP:std}, as $p^{*}$, and the minimum value of the dual LP, in \eqref{LP:dual}, as $m^{*}$. The following property is called \emph{weak duality} (see \cite{boyd}):

\begin{proposition}
	It holds that $p^{*}\leq m^{*}$. Hence, for any feasible point of the dual LP, $\tilde{\mathbf{u}}$, such that $A^T\tilde{\mathbf{u}} \succcurlyeq \mathbf{c}$, with value $\mathbf{b}^T\tilde{\mathbf{u}} =: \tilde{m}$, we have that $p^{*}\leq \tilde{m}$. 
\end{proposition}

We shall now pick a feasible point, $\tilde{\mathbf{u}}$, such that its value, $\tilde{m}$, is equal to $\frac{1}{d+1}$. 

Note that the co-ordinates of $\tilde{\mathbf{u}}$ correspond to the constraints in the primal LP. Let $\tilde{u}(1) = \frac{1}{d+1}$. 

For $i\in \{2,\ldots,|\mathscr{S}\times \mathscr{V}^{(d)}|+1\}$, we identify the co-ordinate $\tilde{u}(i)$ by the node, $(s,v)$, in $\mathscr{G}_{SQ}^{(d)}$, the stationarity constraint of which it corresponds to, i.e., we write $\tilde{u}(i)\equiv \tilde{u}(s,v)$, for a particular $(s,v)$. We then set $\tilde{u}(0,v) = \frac{d}{d+1}$, and $\tilde{u}(s,v) = \frac{d-1}{d+1}$, for $s\neq d$. All other co-ordinates of $\tilde{\mathbf{u}}$ are set to $0$.

We only need to verify now that $A^T\tilde{\mathbf{u}} \succcurlyeq \mathbf{c}$. If this holds, then $\tilde{m} = \mathbf{b}^T\tilde{\mathbf{u}} = \tilde{u}(1)=\frac{1}{d+1}$. 

Let us index the rows of $A^T$ by the edge variables they correspond to, i.e., the rows of $A^T$ are written as $\mathbf{a}^T(s,v,x,y)$, for $(s,v,x,y)\in \mathscr{S}\times \mathscr{V}^{(d)}\times \mathscr{X}\times \mathscr{Y}$. Owing to our definition of $\mathbf{\tilde{u}}$, we note that it is sufficient to consider those co-ordinates, $i$, of $\mathbf{a}^T(s,v,x,y)$ such that $i\in [|\mathscr{S}\times \mathscr{V}^{(d)}|+1]$. As was done earlier, in the evaluation of $\mathbf{a}^T(s,v,x,y)\tilde{\mathbf{u}}$ that follows, we shall identify the index $i\in [2:|\mathscr{S}\times \mathscr{V}^{(d)}|+1]$ corresponding to a co-ordinate of $\mathbf{a}^T(s,v,x,y)$ by the node, $(s,v)$, of $\mathscr{G}_{SQ}^{(d)}$, the stationarity constraint of which it corresponds to. 

\begin{enumerate}
	\item $(s,v,x,y) = (0,v,0,y)$, for $y\in \{0,?\}$: In this case, $\mathbf{a}^T(s,v,x,y)$ has $1$s in the first co-ordinate (corresponding to the PMF constraint) and in the co-ordinates corresponding to the index $(1,v^+)$, for $v^+ = \Phi(v,y)$, and $-1$ in the co-ordinate corresponding to the index $(0,v)$. We then have that
	\begin{align}\label{eq:eval1}
	\mathbf{a}^T(s,v,x,y)\tilde{\mathbf{u}} &= \frac{1}{d+1}+\frac{d-1}{d+1}-\frac{d}{d+1}\notag\\ &=0.
	\end{align}
	\item $(s,v,x,y) = (\hat{s},v,0,y)$, for $\hat{s}\notin \{0,d\}$, $y\in \{0,?\}$: Here, $\mathbf{a}^T(s,v,x,y)$ has $1$s in the first (PMF) co-ordinate and in the co-ordinates corresponding to the index $(\hat{s}+1,v^+)$, for $v^+ = \Phi(v,y)$, and $-1$ in the co-ordinate corresponding to the index $(\hat{s},v)$. It then holds that 
	\begin{align}\label{eq:eval2}
	\mathbf{a}^T(s,v,x,y)\tilde{\mathbf{u}} &= \frac{1}{d+1}+\frac{d-1}{d+1}-\frac{d-1}{d+1}\notag\\ &=\frac{1}{d+1}.
	\end{align}
	\item $(s,v,x,y) = (d,\mathbf{q},0,y)$, for $\mathbf{q}\in \mathscr{V}_{\text{DB}}^{(d)}$, $y\in \{0,?\}$: In this case, $\mathbf{a}^T(s,v,x,y)$ has $1$s in the first (PMF) co-ordinate and in the co-ordinates corresponding to the index $(d,\mathbf{q}^+)$, for $\mathbf{q}^+ = \Phi(\mathbf{q},y)$, and $-1$ in the co-ordinate corresponding to the index $(d,\mathbf{q})$. We then have that
	\begin{align}\label{eq:eval3}
	\mathbf{a}^T(s,v,x,y)\tilde{\mathbf{u}} = \frac{1}{d+1}.
	\end{align}
	\item $(s,v,x,y) = (d,\mathbf{q},1,y)$, for $y\in \{0,?\}$: For this final class of edges, $\mathbf{a}^T(s,v,x,y)$ has $1$s in the first (PMF) co-ordinate and in the co-ordinates corresponding to the index $(0,Q_0)$, since $Q_0 = \Phi(\mathbf{q},y)$, and $-1$ in the co-ordinate corresponding to the index $(d,\mathbf{q})$. It is then true that
	\begin{align}\label{eq:eval4}
	\mathbf{a}^T(s,v,x,y)\tilde{\mathbf{u}} &= \frac{1}{d+1}+\frac{d}{d+1}\notag\\ &=1.
	\end{align}
\end{enumerate}
From equations \eqref{eq:eval1}, \eqref{eq:eval2}, \eqref{eq:eval3}, and \eqref{eq:eval4}, and from the definition of $\mathbf{c}$, it follows that $A^T\tilde{\mathbf{u}} \succcurlyeq \mathbf{c}$, and, hence, $\tilde{m} = \frac{1}{d+1}\geq p^{*}$, thereby proving the proposition.

\end{proof}
